# Supplementary material for: A Framework for Combining Entity Resolution and Query Answering in Knowledge Bases
Source: arXiv:2303.07469 source file (2023-03-13)
Supplement: Supplementary file 1 [file appendix.tex]

\newcommand{\Body}{\textsf{body}}

\begin{appendices}

\section{Chase}

We now show a complete execution of the chase procedure in our ongoing example. In the following, we use $\Body(r)$ to the note the body of a rule $r$.

\begin{example}
    \nb{missing notation of body}
    \label{ex:chase_full_example}
    Consider the KB $\K=\tup{\T,\DB}$ in the Example~\ref{ex:query}. 
    We report in the following the rules composing $\T$ for the sake of presentation:
	\begin{align*}
		\arraycolsep=0.3pt
		\begin{array}{ll}
			r_1) & \Emp(p,\comp) \rightarrow \Pers(p)    					\\
			r_2) & \CI(p, \name_1, \phone_1) \wedge \CI(p, \name_2, \phone_2)\\ 
                 &   \rightarrow \name_1 = \name_2 \\
            r_3) & \CI(p,\name_1,\phone_1)\wedge \CI(p,\name_2,\phone_2)\\ 
                 &  \rightarrow \phone_1=\phone_2 \\
            r_4) & \CI(p_1,\name,\phone)\wedge \CI(p_2,\name,\phone) \rightarrow p_1=p_2 \\
			r_5) & \Pers(p_1) \wedge \Pers(p_2) \wedge \Emp(p_1,\comp) \wedge \Emp(p_2,\comp) \wedge\\ 
                 &  \CI(p_1,\name_1,\phone_1) \wedge \CI(p_2,\name_2,\phone_2) \wedge\\
		         &   \JaccardSim(\name_1,\name_2,0.6) \rightarrow p_1 = p_2\\
            r_6) & \Emp(p,\comp) \rightarrow \CEO(\comp,\director) \wedge \Pers(\director) \\
            r_7) & \CEO(\comp,\director_1) \wedge \CEO(\comp,\director_2) \\
            & \rightarrow \director_1 = \director_2
		\end{array}
	\end{align*}    
 Let now $\I^\DB$ the \emph{base instance} composed by the following facts:\nb{It would be preferable to align the order of the facts to the order of the ground atoms in $\DB$ of Example 2. That is $d_4 -> d_6$, $d_6 -> d_7$, $d_7 -> d_4$. The other steps must be modified accordingly.}
    \begin{align*}
		\arraycolsep=3.0pt
		\begin{array}{ll}
			d_1) & \Emp([\Doe_1], [\Yahoo]) \\
			d_2) & \Emp([\Doe_2], [\Yahoo]) \\
			d_3) & \Emp([\Doe_3], [\IBM]) \\
            d_4) & \CI([\Doe_3], \{ \texttt{Mary Doe} \}, \{ \PNumberA \}) \\
            d_5) & \CI([\Doe_2], \{ \texttt{John Doe} \}, \{ \PNumberB \}) \\
            d_6) & \CI([\Doe_4], \{ \texttt{J. Doe}\}, \{ \PNumberB\}) \\
			d_7) & \CI([\Doe_1], \{ \texttt{J. Doe} \}, \{ \PNumberA \}) \\ 
            d_8) & \CEO([\Yahoo],[\Doe_1]) \\
		\end{array}
	\end{align*}
    One possible chase sequence can be the one composed by the following chase steps:
   
    \smallskip
    \noindent
    \textbf{Step 1:} $\I_D \xrightarrow[]{r_6,\mu_0} \I_1$,
    %The result of applying $r_6$ to $\I_D$ with the assignment $\mu_0$ from \Body($r_6$) to $\I_D$ such that %$\mu_0(\Body(r_6))= \{ d_1 \}$, is the new instance $\I_1$ composed by the following facts:
    where $\mu_0$ is such that $\mu_0(\Body(r_6))= \{ d_1 \}$. The resulting instance $\I_1$ contains the facts $d_1$-$d_8$ plus the following facts:
    \begin{align*}
		\arraycolsep=3.0pt
		\begin{array}{ll}
%			d_1) & \Emp([\Doe_1], [\Yahoo]) \\
%			d_2) & \Emp([\Doe_2], [\Yahoo]) \\
%			d_3) & \Emp([\Doe_3], [\IBM]) \\
%            d_4) & \CI([\Doe_3], \{ \texttt{Mary Doe} \}, \{ \PNumberA \}) \\
%            d_5) & \CI([\Doe_2], \{ \texttt{John Doe} \}, \{ \PNumberB \}) \\
%            d_6) & \CI([\Doe_4], \{ \texttt{J. Doe}\}, \{ \PNumberA\}) \\
%			d_7) & \CI([\Doe_1], \{ \texttt{J. Doe} \}, \{ \PNumberB \}) \\ 
%            d_8) & \CEO([\Yahoo],[\Doe_1]) \\
            d_9) & \CEO([\Yahoo],[\textnormal{\textbf{e}}_1^\bot]) \\
            d_{10}) & Pers([\textnormal{\textbf{e}}_1^\bot])
		\end{array}
	\end{align*}
    \noindent \textbf{Step 2:} $\I_1 \xrightarrow[]{r_7,\mu_1} \I_2$,
    %The result of applying $r_7$ to $\I_1$ with the assignment $\mu_1$ from \Body($r_7$) to $\I_1$ such that $\mu_1(\Body(r_6))= \{ d_8, d_9 \}$, is the new instance $\I_2$ composed by the following facts:
    where $\mu_1$ is such that $\mu_1(\Body(r_6))= \{ d_8, d_9 \}$. The resulting instance $\I_2$ contains the facts $d_2$-$d_6$ plus the following facts:
    \begin{align*}
		\arraycolsep=3.0pt
		\begin{array}{ll}
			d_{11}) & \Emp([\Doe_1,\textnormal{\textbf{e}}_1^\bot], [\Yahoo]) \\
%			d_2) & \Emp([\Doe_2], [\Yahoo]) \\
%			d_3) & \Emp([\Doe_3], [\IBM]) \\
%           d_4) & \CI([\Doe_3], \{ \texttt{Mary Doe} \}, \{ \PNumberA \}) \\
%           d_5) & \CI([\Doe_2], \{ \texttt{John Doe} \}, \{ \PNumberB \}) \\
%           d_6) & \CI([\Doe_4], \{ \texttt{J. Doe}\}, \{ \PNumberA\}) \\
			d_{12}) & \CI([\Doe_1,\textnormal{\textbf{e}}_1^\bot], \{ \texttt{J. Doe} \}, \{ \PNumberA \}) \\ 
            d_{13}) & \CEO([\Yahoo],[\Doe_1,\textnormal{\textbf{e}}_1^\bot]) \\
            d_{14}) & Pers([\Doe_1,\textnormal{\textbf{e}}_1^\bot])
		\end{array}
	\end{align*}
%    Note that we deleted $d_8$ which is the same as $d_9$ after propagating the replace of the newly discovered equivalence class over the new produced instance.
    Note that $d_{13}$ replaces facts $d_8$ and $d_9$ of $\I_1$.
    
    \smallskip
    \noindent
    \textbf{Step 3:} $\I_2 \xrightarrow[]{r_1,\mu_2} \I_3$,
 %   The result of applying $r_1$ to $\I_2$ with the assignment $\mu_2$ from \Body($r_1$) to $\I_2$ such that $\mu_2(\Body(r_1))= \{ d_2 \}$, is the new instance $\I_3$ composed by the following facts:
    where $\mu_2$ is such that $\mu_2(\Body(r_1))= \{ d_2 \}$. The resulting instance $\I_3$ contains the facts $d_2$-$d_6$, $d_{11}$-$d_{14}$ plus the fact
    \begin{align*}
		\arraycolsep=3.0pt
		\begin{array}{ll}
%			d_1) & \Emp([\Doe_1,\textnormal{\textbf{e}}_1^\bot], [\Yahoo]) \\
%			d_2) & \Emp([\Doe_2], [\Yahoo]) \\
%			d_3) & \Emp([\Doe_3], [\IBM]) \\
%            d_4) & \CI([\Doe_3], \{ \texttt{Mary Doe} \}, \{ \PNumberA \}) \\
%            d_5) & \CI([\Doe_2], \{ \texttt{John Doe} \}, \{ \PNumberB \}) \\
%            d_6) & \CI([\Doe_4], \{ \texttt{J. Doe}\}, \{ \PNumberA\}) \\
%			d_7) & \CI([\Doe_1,\textnormal{\textbf{e}}_1^\bot], \{ \texttt{J. Doe} \}, \{ \PNumberB \}) \\ 
%            d_9) & \CEO([\Doe_1,\textnormal{\textbf{e}}_1^\bot],[\Yahoo]) \\
%            d_{10}) & Pers([\Doe_1,\textnormal{\textbf{e}}_1^\bot]) \\
            d_{15}) & Pers([\Doe_2])
		\end{array}
	\end{align*}
    
    \smallskip
    \noindent
    \textbf{Step 4:} $\I_3 \xrightarrow[]{r_1,\mu_3} \I_4$,
   % The result of applying $r_1$ to $\I_1$ with the assignment $\mu_3$ from \Body($r_1$) to $\I_3$ such that $\mu_3(\Body(r_1))= \{ d_3 \}$, is the new instance $\I_4$ composed by the following facts:
    where $\mu_3$ is such that $\mu_3(\Body(r_1))= \{ d_3 \}$. The resulting instance $\I_4$ contains the facts $d_2$-$d_6$, $d_{11}$-$d_{15}$ plus the fact
    \begin{align*}
		\arraycolsep=3.0pt
		\begin{array}{ll}
%			d_1) & \Emp([\Doe_1,\textnormal{\textbf{e}}_1^\bot], [\Yahoo]) \\
%			d_2) & \Emp([\Doe_2], [\Yahoo]) \\
%			d_3) & \Emp([\Doe_3], [\IBM]) \\
%            d_4) & \CI([\Doe_3], \{ \texttt{Mary Doe} \}, \{ \PNumberA \}) \\
%            d_5) & \CI([\Doe_2], \{ \texttt{John Doe} \}, \{ \PNumberB \}) \\
%            d_6) & \CI([\Doe_4], \{ \texttt{J. Doe}\}, \{ \PNumberA\}) \\
%			d_7) & \CI([\Doe_1,\textnormal{\textbf{e}}_1^\bot], \{ \texttt{J. Doe} \}, \{ \PNumberB \}) \\ 
%            d_9) & \CEO([\Doe_1,\textnormal{\textbf{e}}_1^\bot],[\Yahoo]) \\
%            d_{10}) & Pers([\Doe_1,\textnormal{\textbf{e}}_1^\bot]) \\
%            d_{11}) & Pers([\Doe_2]) \\
            d_{16}) & Pers([\Doe_3])
		\end{array}
	\end{align*}
    
    \smallskip
    \noindent
    \textbf{Step 5} $\I_4 \xrightarrow[]{r_5,\mu_4} \I_5$,
  %  The result of applying $r_5$ to $\I_4$ with the assignment $\mu_4$ from \Body($r_5$) to $\I_4$ such that $\mu_4(\Body(r_5))= \{ d_1, d_2, d_5, d_7 \}$, is the new instance $\I_5$ composed by the following facts:
  where $\mu_4$ is such that $\mu_4(\Body(r_5))$ is the set $\{ d_{14}, d_{15}, d_{11}, d_2, d_{12}, d_5 \}$ plus the fact $\JaccardSim(\{\texttt{J. Doe}\},\{\texttt{John Doe}\},\{0.6\})$. The resulting instance $\I_5$ is as follows:
    \begin{align*}
		\arraycolsep=3.0pt
		\begin{array}{ll}
			d_{17}) & \Emp([\Doe_1, \Doe_2,\textnormal{\textbf{e}}_1^\bot], [\Yahoo]) \\
			d_3) & \Emp([\Doe_3], [\IBM]) \\
            d_4) & \CI([\Doe_3], \{ \texttt{Mary Doe} \}, \{ \PNumberA \}) \\
            d_{18}) & \CI([\Doe_1, \Doe_2,\textnormal{\textbf{e}}_1^\bot], \\ & \hfill \{ \texttt{John Doe} \}, \{ \PNumberB \}) \\
            d_6) & \CI([\Doe_4], \{ \texttt{J. Doe}\}, \{ \PNumberA\}) \\
			d_{19}) & \CI([\Doe_1, \Doe_2,\textnormal{\textbf{e}}_1^\bot], \\ & \hfill \{ \texttt{J. Doe} \}, \{ \PNumberA \}) \\ 
            d_{20}) & \CEO([\Doe_1, \Doe_2,\textnormal{\textbf{e}}_1^\bot], [\Yahoo]) \\
            d_{21}) & Pers([\Doe_1, \Doe_2,\textnormal{\textbf{e}}_1^\bot]) \\
            d_{16}) & Pers([\Doe_3])
		\end{array}
	\end{align*}
   % Note that we removed $d_2$ and $d_{10}$ such that they were equal to other facts in the Instance.
     Note that $d_{17}$ replaces facts $d_2$ and $d_{11}$ of $\I_4$, and $d_{21}$ replaces facts $d_{14}$ and $d_{15}$ of $\I_4$.
     
    \smallskip
    \noindent
    \textbf{Step 6:} $\I_5 \xrightarrow[]{r_2,\mu_5} \I_6$,
   % The result of applying $r_2$ to $\I_5$ with the assignment $\mu_5$ from \Body($r_2$) to $\I_5$ such that $\mu_5(\Body(r_2))= \{ d_5, d_7 \}$, is the new instance $\I_6$ composed by the following facts:
   where $\mu_5$ is such that $\mu_5(\Body(r_2))= \{ d_{18}, d_{19} \}$. The resulting instance $\I_6$ is as follows:
    \begin{align*}
		\arraycolsep=3.0pt
		\begin{array}{ll}
			d_{17}) & \Emp([\Doe_1, \Doe_2,\textnormal{\textbf{e}}_1^\bot], [\Yahoo]) \\
			d_{3}) & \Emp([\Doe_3], [\IBM]) \\
            d_{4}) & \CI([\Doe_3], \{ \texttt{Mary Doe} \}, \{ \PNumberA \}) \\
            d_{22}) & \CI([\Doe_1, \Doe_2,\textnormal{\textbf{e}}_1^\bot], \\ &  \hspace{1.5cm} \{ \texttt{John Doe}, \texttt{J. Doe} \}, \{ \PNumberB \}) \\
            d_6) & \CI([\Doe_4], \{ \texttt{J. Doe}\}, \{ \PNumberA\}) \\
            d_{23}) & \CI([\Doe_1, \Doe_2,\textnormal{\textbf{e}}_1^\bot], \\ &  \hfill \{ \texttt{John Doe}, \texttt{J. Doe} \}, \{ \PNumberA \}) \\
            d_{20}) & \CEO([\Doe_1, \Doe_2,\textnormal{\textbf{e}}_1^\bot], [\Yahoo]) \\
            d_{21}) & Pers([\Doe_1, \Doe_2,\textnormal{\textbf{e}}_1^\bot]) \\
            d_{16}) & Pers([\Doe_3])
		\end{array}
	\end{align*}
    
    \smallskip
    \noindent
    \textbf{Step 7:} $\I_6 \xrightarrow[]{r_3,\mu_6} \I_7$,
  %  The result of applying $r_3$ to $\I_6$ with the assignment $\mu_6$ from \Body($r_3$) to $\I_6$ such that $\mu_6(\Body(r_3))= \{ d_5, d_7 \}$, is the new instance $\I_7$ composed by the following facts: \nb{non-Empty inters}
    where $\mu_6$ is such that $\mu_6(\Body(r_3))= \{ d_{22}, d_{23} \}$. The resulting instance $\I_7$ is as follows:
    \begin{align*}
		\arraycolsep=3.0pt
		\begin{array}{ll}
			d_{17}) & \Emp([\Doe_1, \Doe_2,\textnormal{\textbf{e}}_1^\bot], [\Yahoo]) \\
			d_3) & \Emp([\Doe_3], [\IBM]) \\
            d_4) & \CI([\Doe_3], \{ \texttt{Mary Doe} \}, \{ \PNumberA \}) \\
            d_{24}) & \CI([\Doe_1, \Doe_2,\textnormal{\textbf{e}}_1^\bot], \{ \texttt{John Doe}, \texttt{J. Doe} \}, \\ & \{ \PNumberA , \PNumberB \}) \\ 
            d_6) & \CI([\Doe_4], \{ \texttt{J. Doe}\}, \{ \PNumberA \}) \\
            d_{20}) & \CEO([\Doe_1, \Doe_2,\textnormal{\textbf{e}}_1^\bot],[\Yahoo]) \\
            d_{21}) & Pers([\Doe_1, \Doe_2,\textnormal{\textbf{e}}_1^\bot]) \\
            d_{16}) & Pers([\Doe_3])
		\end{array}
	\end{align*}
    Note that $d_{24}$ replaces facts $d_{22}$ and $d_{23}$ of $\I_6$.
    
    \smallskip
    \noindent
    \textbf{Step 8:} $\I_7 \xrightarrow[]{r_4,\mu_7} \I_8$,
   % The result of applying $r_3$ to $\I_7$ with the assignment $\mu_7$ from \Body($r_4$) to $\I_7$ such that $\mu_7(\Body(r_4))= \{ d_6, d_7 \}$, is the new instance $\I_8$ composed by the following facts:
   where $\mu_7$ is such that $\mu_7(\Body(r_4))= \{ d_{24}, d_{6} \}$. The resulting instance $\I_8$ is as follows:\nb{this is the only step in which we use (twice) non-empty intersection of sets of values in the assignment.}
    \begin{align*}
		\arraycolsep=3.0pt
		\begin{array}{ll}
			d_{25}) & \Emp([\Doe_1, \Doe_2, \Doe_4, \textnormal{\textbf{e}}_1^\bot], [\Yahoo]) \\
			d_3) & \Emp([\Doe_3], [\IBM]) \\
            d_4) & \CI([\Doe_3], \{ \texttt{Mary Doe} \}, \{ \PNumberA \}) \\
            d_{26}) & \CI([\Doe_1, \Doe_2, \Doe_4, \textnormal{\textbf{e}}_1^\bot], \\ & \{ \texttt{John Doe}, \texttt{J. Doe} \}, \{ \PNumberA , \PNumberB \}) \\ 
            d_{27}) & \CI([\Doe_1, \Doe_2, \Doe_4, \textnormal{\textbf{e}}_1^\bot], \{ \texttt{J. Doe}\}, \{ \PNumberA\}) \\
            d_{28}) & \CEO([\Doe_1, \Doe_2, \Doe_4, \textnormal{\textbf{e}}_1^\bot], [\Yahoo]) \\
            d_{29}) & Pers([\Doe_1, \Doe_2, \Doe_4, \textnormal{\textbf{e}}_1^\bot]) \\
            d_{16}) & Pers([\Doe_3])
		\end{array}
	\end{align*}
 
    \smallskip
    \noindent
    \textbf{Step 9:} $\I_8 \xrightarrow[]{r_3,\mu_8} \I_9$,
   % The result of applying $r_3$ to $\I_8$ with the assignment $\mu_8$ from \Body($r_3$) to $\I_8$ such that $\mu_8(\Body(r_3))= \{ d_6, d_7 \}$, is the new instance $\I_9$ composed by the following facts: \nb{non-Empty intersction show S...}
   where $\mu_8$ is such that $\mu_7(\Body(r_3))= \{ d_{26}, d_{27} \}$. The resulting instance $\I_8$ is as follows
    \begin{align*}
		\arraycolsep=3.0pt
		\begin{array}{ll}
			d_{25}) & \Emp([\Doe_1, \Doe_2, \Doe_4, \textnormal{\textbf{e}}_1^\bot], [\Yahoo]) \\
			d_3) & \Emp([\Doe_3], [\IBM]) \\
            d_4) & \CI([\Doe_3], \{ \texttt{Mary Doe} \}, \{ \PNumberA \}) \\
			d_{26}) & \CI([\Doe_1, \Doe_2, \Doe_4, \textnormal{\textbf{e}}_1^\bot], \\ & \{ \texttt{John Doe}, \texttt{J. Doe} \}, \{ \PNumberA , \PNumberB \}) \\ 
            d_{30}) & \CI([\Doe_1, \Doe_2, \Doe_4, \textnormal{\textbf{e}}_1^\bot], \{ \texttt{J. Doe}\}, \\ & \{ \PNumberA , \PNumberB \}) \\
            d_{28}) & \CEO([\Doe_1, \Doe_2, \Doe_4, \textnormal{\textbf{e}}_1^\bot], [\Yahoo]) \\
            d_{29}) & Pers([\Doe_1, \Doe_2, \Doe_4, \textnormal{\textbf{e}}_1^\bot]) \\
            d_{16}) & Pers([\Doe_3])
		\end{array}
	\end{align*}
    
    \smallskip
    \noindent
    \textbf{Step 10:} $\I_9 \xrightarrow[]{r_2,\mu_9} \I_{10}$,
   % The result of applying $r_2$ to $\I_9$ with the assignment $\mu_9$ from \Body($r_2$) to $\I_9$ such that $\mu_9(\Body(r_2))= \{ d_6, d_7 \}$, is the new instance $\I_{10}$ composed by the following facts:
   where $\mu_9$ is such that $\mu_9(\Body(r_2))= \{ d_{26}, d_{30} \}$. The resulting instance $\I_{10}$ is as follows
    \begin{align*}
		\arraycolsep=3.0pt
		\begin{array}{ll}
			d_{25}) & \Emp([\Doe_1, \Doe_2, \Doe_4, \textnormal{\textbf{e}}_1^\bot], [\Yahoo]) \\
			d_3) & \Emp([\Doe_3], [\IBM]) \\
            d_4) & \CI([\Doe_3], \{ \texttt{Mary Doe} \}, \{ \PNumberA \}) \\
			d_{26}) & \CI([\Doe_1, \Doe_2, \Doe_4, \textnormal{\textbf{e}}_1^\bot], \\ & \{ \texttt{John Doe}, \texttt{J. Doe} \}, \{ \PNumberA , \PNumberB \}) \\ 
            d_{28}) & \CEO([\Doe_1, \Doe_2, \Doe_4, \textnormal{\textbf{e}}_1^\bot], [\Yahoo]) \\
            d_{29}) & Pers([\Doe_1, \Doe_2, \Doe_4, \textnormal{\textbf{e}}_1^\bot]) \\
            d_{16}) & Pers([\Doe_3])
		\end{array}
	\end{align*}
    Note that we simply removed $d_{30}$ because the chase step replaces it with a fact coinciding with $d_{26}$.

    It is not difficult to see that no rule of $\T$ can be applied to $\I_{10}$, and thus the chase procedure terminates. The result of the chase is indeed $\I_{10}$ \qed

\end{example}

\end{appendices}
